# Supplementary material for: Exploiting Multiple EEG Data Domains with Adversarial Learning
Source: arXiv:2204.07777 source file (2022-04-16)
Supplement: Supplementary file 1 [file 07appendix.tex]

\appendix
\section{Specifications of the used neural network encoder.}\label{apd:used-implementations}

\begin{table}[h!]
    \centering
    \caption{DeepConvNet encoder architecture}
    \label{tab:DeepConvNetImplementation}
    \begin{tabular}{p{0.3\textwidth}p{0.7\textwidth}}
    \toprule
    Layer & Details / Parameters \\
    \midrule
         Conv2D & number of filters: 25, kernel size: $1 \times 5$, bias: Yes \\
         Conv2D & number of filters: 25, kernel size: $C \times 1$, bias: No \\
         BatchNormalization & epsilon: 1e-05, momentum: 0.1 \\
         Activation & Exponential Linear Unit \\
         MaxPooling2D & poolsize: $1 \times 2$, strides: $1 \times 2$\\
         Dropout & probability: $50\%$\\
         Conv2D & number of filters: 50, kernel size: $1 \times 4$, bias: No \\
         BatchNormalization & epsilon: 1e-05, momentum: 0.1 \\
         Activation & Exponential Linear Unit \\
         MaxPooling2D & poolsize: $1 \times 2$, strides: $1 \times 2$\\
         Dropout & probability: $50\%$\\
         Conv2D & number of filters: 100, kernel size: $1 \times 5$, bias: No \\
         BatchNormalization & epsilon: 1e-05, momentum: 0.1 \\
         Activation & Exponential Linear Unit \\
         MaxPooling2D & poolsize: $1 \times 2$, strides: $1 \times 2$\\
         Dropout & probability: $50\%$\\
         Conv2D & number of filters: 200, kernel size: $1 \times 5$, bias: No \\
         BatchNormalization & epsilon: 1e-05, momentum: 0.1 \\
         Activation & Exponential Linear Unit \\
         MaxPooling2D & poolsize: $1 \times 2$, strides: $1 \times 2$\\
         Dropout & probability: $50\%$\\
         Flatten & - \\
         \bottomrule
    \end{tabular}
\end{table}

% Comment from Ozan: I don't think this is necessary, since it is in the text.
%
% \begin{table}[h!]
%     \centering
%     \caption{Used Implementation of the Adversary Network and Emotion Classifier}
%     \label{tab:AdversaryClassifierImplementation}
%     \begin{tabular}{p{0.3\textwidth}p{0.7\textwidth}}
%         \toprule
%          Layer & Details / Parameters \\
%         \midrule
%          Dense & bias: No \\
%          \bottomrule
%     \end{tabular}
% \end{table}
